# Supplementary material for: High Resolution Optical Spectroscopy and Magnetic Properties of Yb3+ in Y2SiO5
Source: arXiv:1606.06937 source file (2016-06-22)
Supplement: Supplementary file 1 [file YbYSO_Suppl_v3.pdf]

# High Resolution Optical Spectroscopy and Magnetic Properties of $Yb^{3+}$ in $Y_2SiO_5$

Sacha Welinski,[1] Alban Ferrier,[1,2] Mikael Afzelius,[3] and Philippe Goldner[1]

[1]*PSL Research University, Chimie ParisTech, CNRS, Institut de Recherche de Chimie Paris, 75005, Paris, France*

[2]*Sorbonne Universités, UPMC Univ Paris 06, Paris 75005, France*

[3]*Group of Applied Physics, University of Geneva, CH-1211 Geneva 4, Switzerland*

(Dated: June 22, 2016)

## I. $^2F_{7/2}(0)$ GROUND STATE g-TENSORS

A fit to the EPR experimental angular variations (Fig. S??) gives the following $^2F_{7/2}(0)$ ground state g-tensors in the $(D_1, D_2, b)$ frame.

$$\boldsymbol{g}_{site1} = \begin{pmatrix} 5.85 & -2.23 & -0.02 \\ -2.23 & -0.70 & 0.50 \\ -0.02 & 0.50 & -0.52 \end{pmatrix}_{(D_1 D_2 b)} \qquad \boldsymbol{g}_{site2} = \begin{pmatrix} -0.63 & 0.54 & 1.26 \\ 0.54 & -0.69 & -0.82 \\ 1.26 & -0.82 & 5.75 \end{pmatrix}_{(D_1 D_2 b)}$$

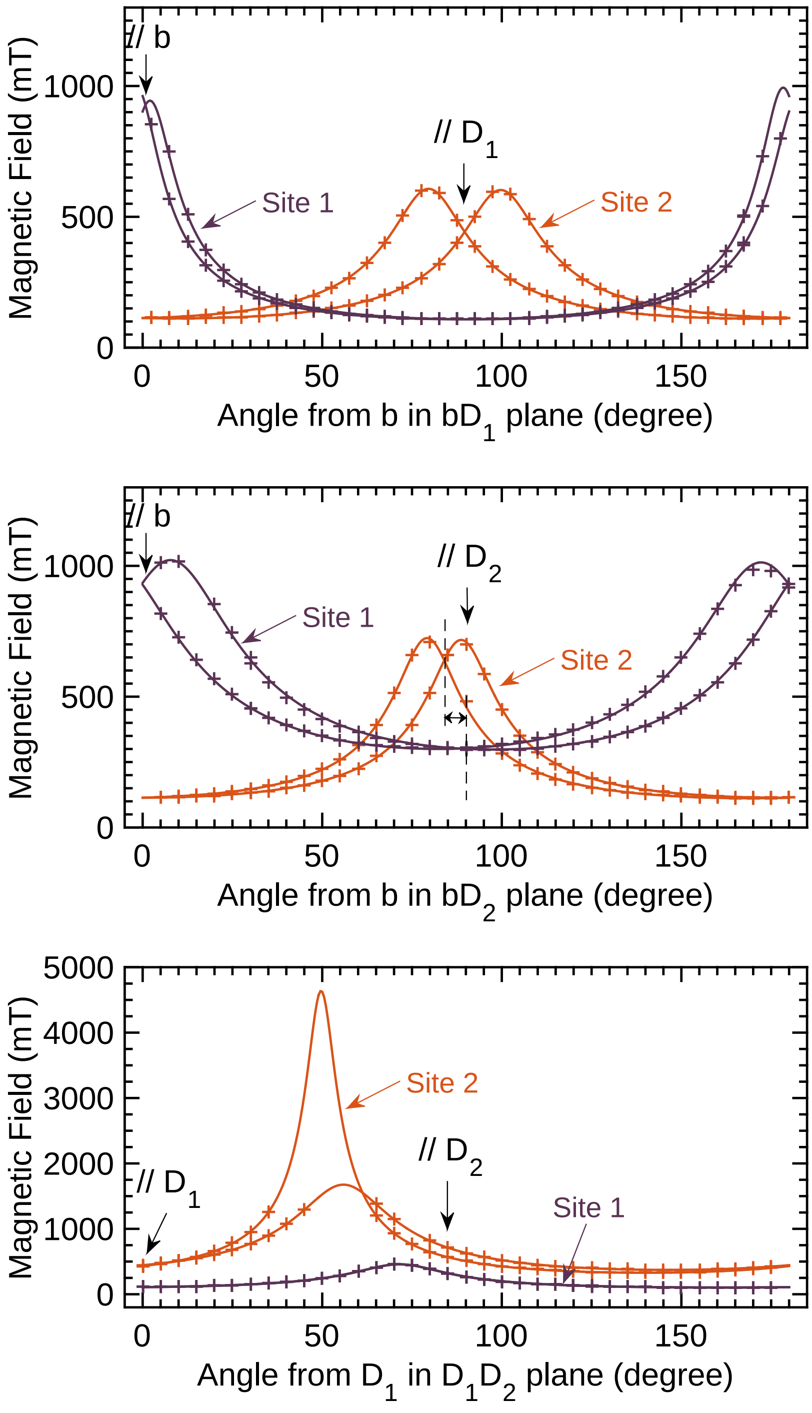


FIG. 1. Angular variation of EPR transitions in the $bD_1$,$bD_2$ and $D_1D_2$ planes ($I = 0$ isotopes) for sites 1 and 2 in $Yb^{3+}$:$Y_2SiO_5$. Crosses: experimental data; lines: fit to a spin Hamiltonian model.

## II. $^2F_{5/2}(0)$ EXCITED STATE g-TENSORS

The ground state g tensors measured by EPR were first compared to the experimental angular variations (Figs. S?? and S??) to check for sample misalignment. The corresponding angles were then used to fit the excited state Zeeman splittings. The $^2F_{5/2}(0)$ excited state state g-tensors in the $(D_1, D_2, b)$ frame are:

$$\boldsymbol{g}_{site1} = \begin{pmatrix} 3.19 & -0.91 & 0.31 \\ -0.91 & -0.54 & 0.15 \\ 0.31 & 0.15 & 1.00 \end{pmatrix}_{(D_1 D_2 b)} \qquad \boldsymbol{g}_{site2} = \begin{pmatrix} -0.32 & -0.86 & -1.21 \\ -0.86 & -0.05 & 1.10 \\ -1.21 & 1.10 & -2.57 \end{pmatrix}_{(D_1 D_2 b)}$$

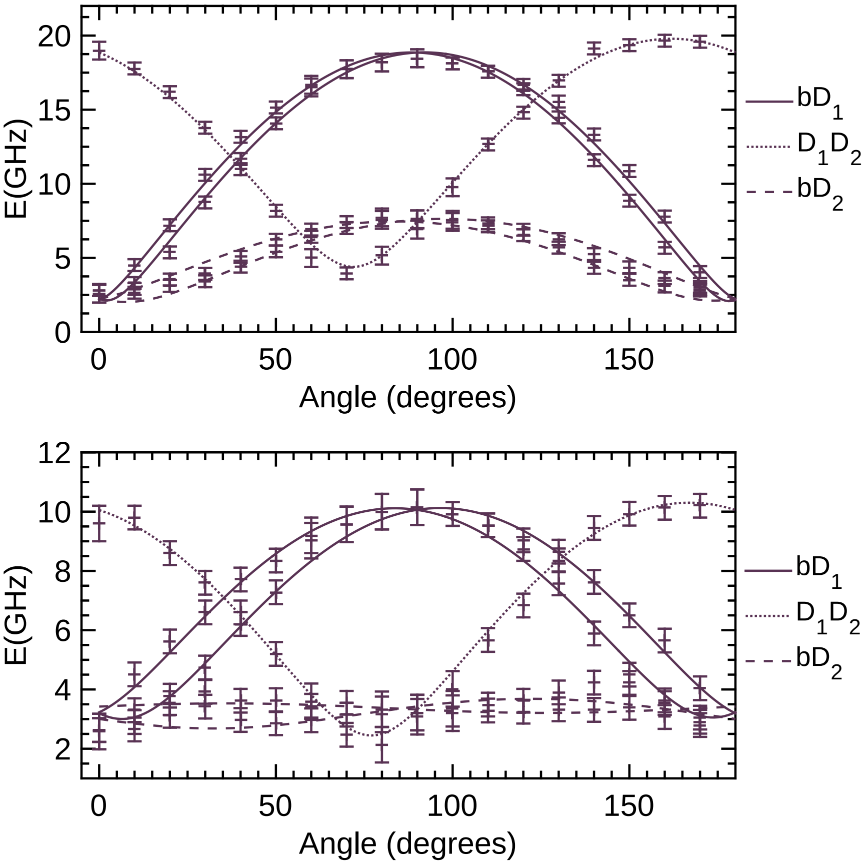


FIG. 2. Angular variation of EPR transitions in the $bD_1$, $bD_2$ and $D_1D_2$ planes ($I = 0$ isotopes) for site 1 in $^2F_{7/2}(0)$ ground state (top) and $^2F_{5/2}(0)$ excited state (bottom) in $Yb^{3+}$:$Y_2SiO_5$ ($B = 217$ mT). Crosses: experimental data; lines: fit to a spin Hamiltonian model.

## III. HYPERFINE STRUCTURES

The $^2F_{7/2}(0)$ ground state state hyperfine tensors for $^{171}Yb^{3+}$ ($I = 1/2$) were determined by a fit to the experimental angular variations (Fig. S**??**) using the $g$ tensors determined for the $I = 0$ isotopes. In the $(D_1, D_2, b)$ frame the $A$ tensors are (in MHz):

$$\boldsymbol{A}_{site1} = \begin{pmatrix} -3844 & 1356 & 1909 \\ 1356 & -2257 & 162 \\ 1909 & 162 & -1340 \end{pmatrix}_{(D_1D_2b)} \qquad \boldsymbol{A}_{site2} = \begin{pmatrix} 1054 & -503 & -894 \\ -503 & 232 & 660 \\ -894 & 660 & -4554 \end{pmatrix}_{(D_1D_2b)}$$

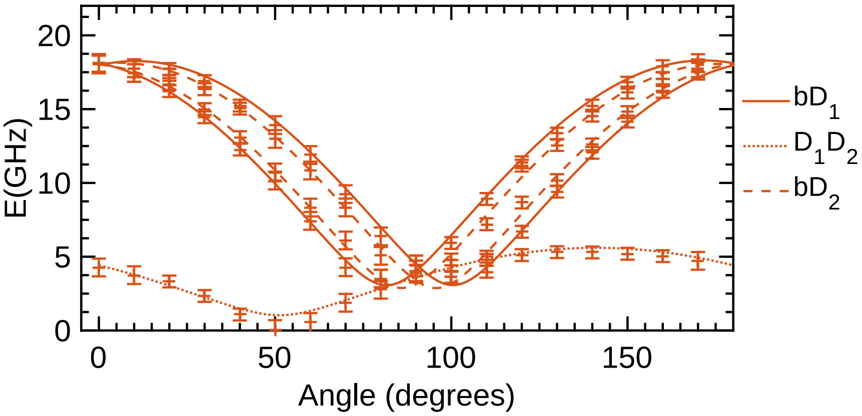


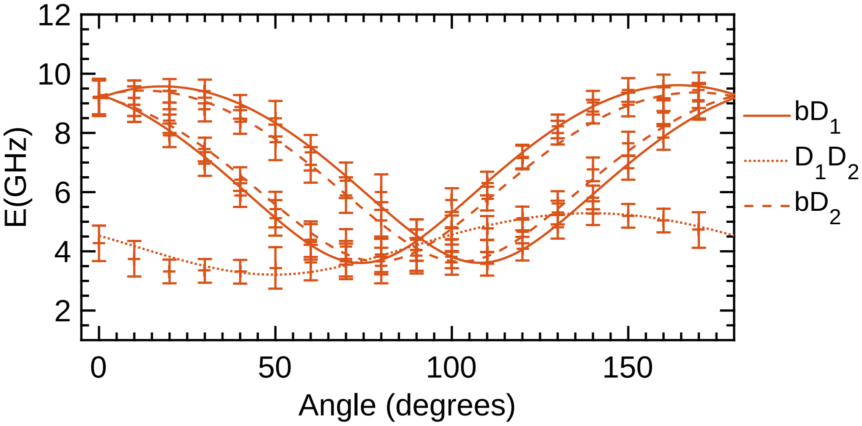


FIG. 3. Angular variation of EPR transitions in the $bD_1$,$bD_2$ and $D_1D_2$ planes ($I = 0$ isotopes) for site 2 in $^2F_{7/2}(0)$ ground state (top) and $^2F_{5/2}(0)$ excited state (bottom) in $Yb^{3+}$:$Y_2SiO_5$ ($B = 217$ mT). Crosses: experimental data; lines: fit to a spin Hamiltonian model.

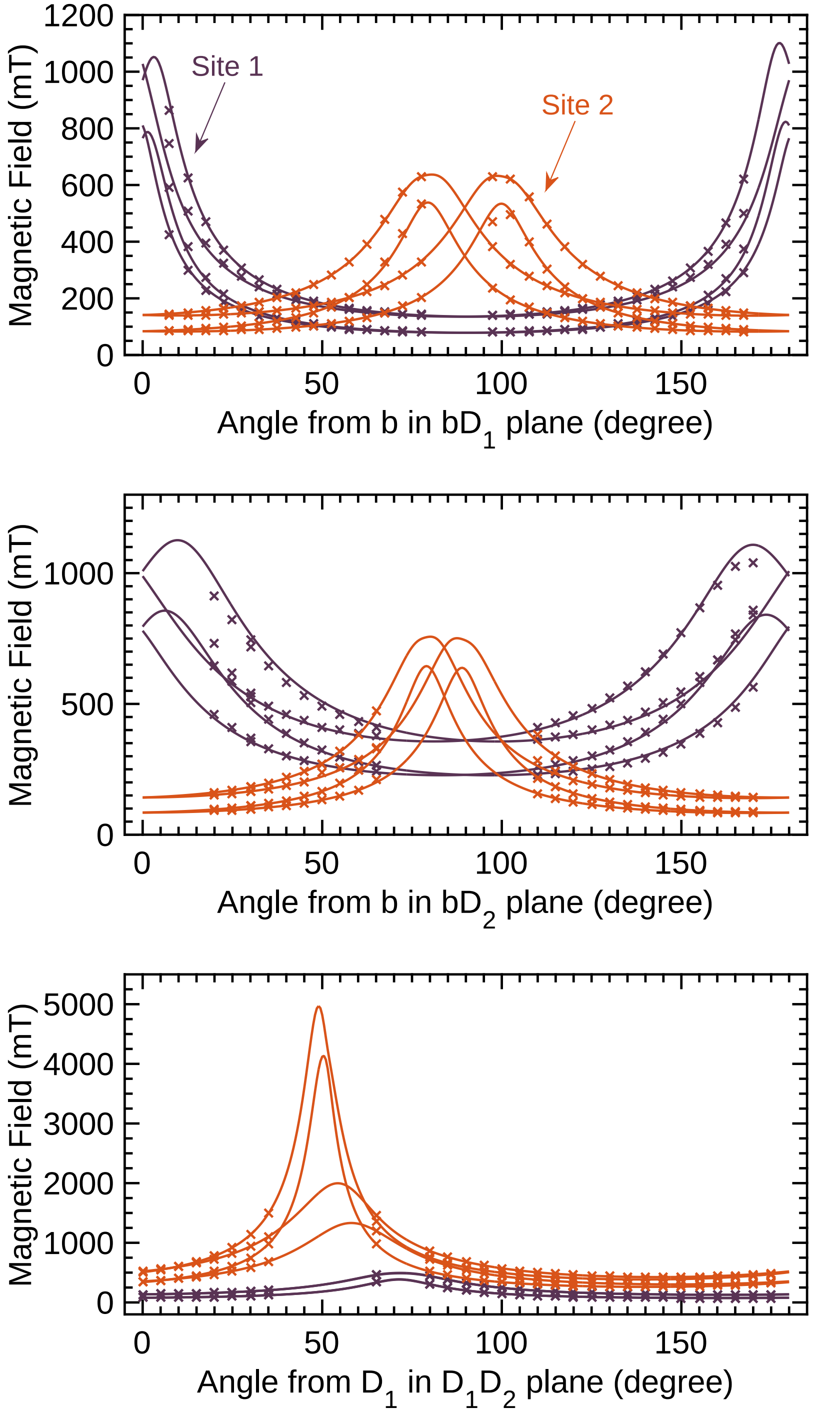


FIG. 4. Angular variations of the EPR transitions of $^{171}Yb^{3+}$ ($I = 1/2$) in the $bD_1$, $bD_2$ and $D_1D_2$ planes for sites 1 and 2. Crosses: experimental data, lines: fit to a spin Hamiltonian model.

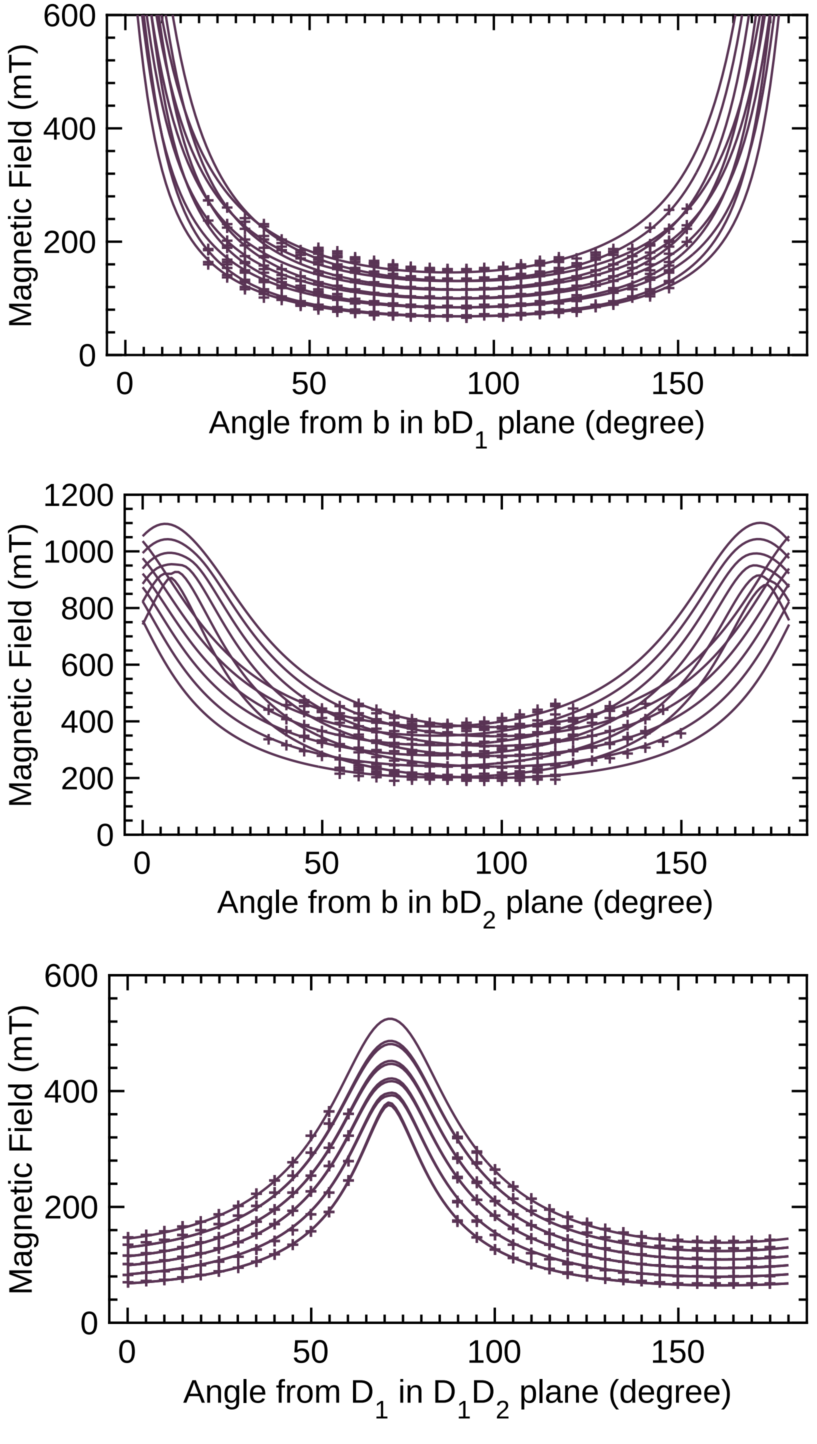


FIG. 5. Angular variations of the strongest EPR transitions of $^{173}Yb^{3+}$ ($I = 5/2$) in the $bD_1$, $bD_2$ and $D_1D_2$ planes in site 1. Crosses: experimental data, lines: calculated fields using $^{171}Yb^{3+}$ $A$ tensor.

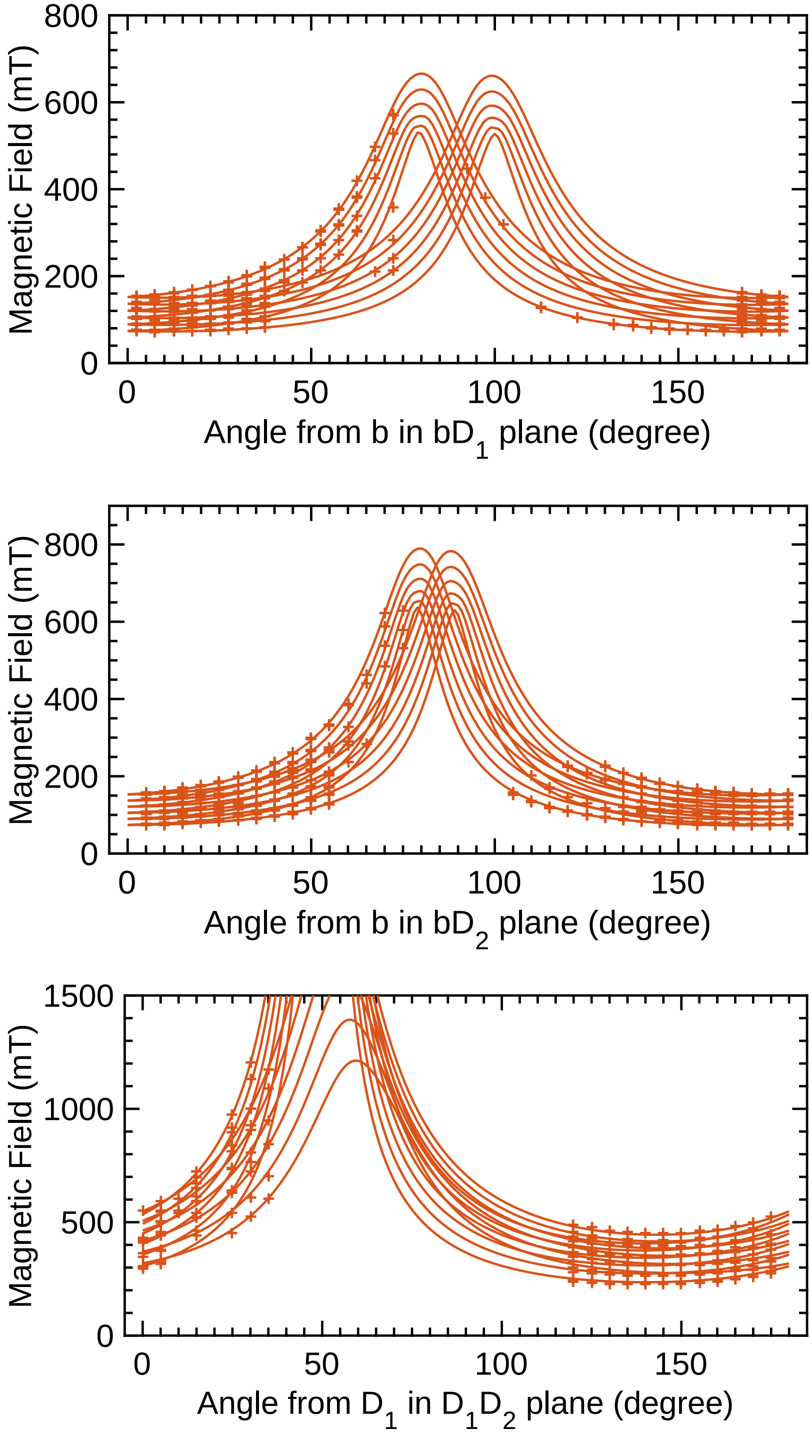


FIG. 6. Angular variations of the strongest EPR transitions of $^{173}Yb^{3+}$ ($I = 5/2$) in the $bD_1$, $bD_2$ and $D_1D_2$ planes in site 2. Crosses: experimental data, lines: calculated fields using $^{171}Yb^{3+}$ $A$ tensor.

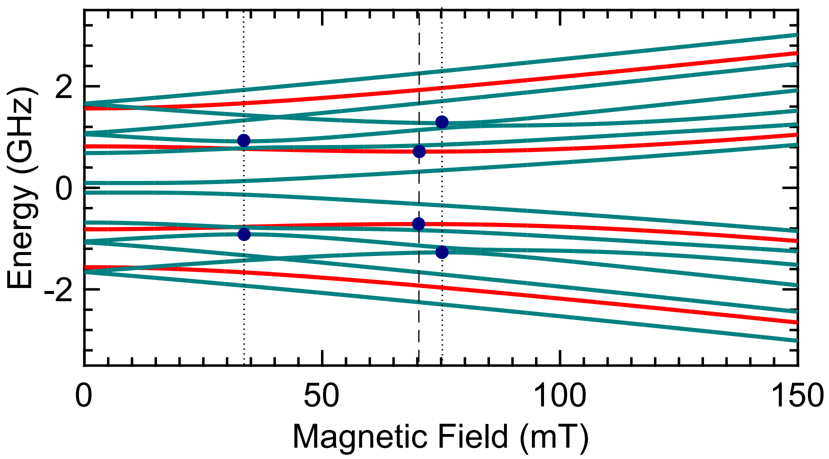


FIG. 7. Calculated energies $E$ of the ground state hyperfine levels of $^{171}Yb^{3+}$($I = 1/2$, red) and $^{173}Yb^{3+}$($I = 5/2$, blue) in site 2 as a function of the magnetic field strength. The field is oriented along $D_1$. The vertical dashed (dotted) line denotes partial clock transitions ($dE/dB$=0) for $I = 1/2$ ($I = 5/2$).
